# Supplementary material for: Generative Parameter Sampler For Scalable Uncertainty Quantification
Source: arXiv:1905.12440 source file (2019-06-02)
Supplement: Supplementary file 1 [file appendix.tex]

\clearpage
\appendix
\onecolumn
\begin{center}
	%\part*{Appendix}
	\Huge \textbf{Appendix}
\end{center}
\addcontentsline{toc}{chapter}{Appendix}
\counterwithin{figure}{section}
\counterwithin{algorithm}{section}
\counterwithin{equation}{section}
\section{Black-Box Variational Inference}
We briefly describe the mechanics of BBVI. To aid discussion, we let $\mathcal{T}=\{T_1,\hdots,T_N\}$ be the observed data and let $\mathcal{Z}=\{\mathcal{Z}1,\hdots,\mathcal{Z}_n\}$ denote a set of latent variables which govern the distribution of data. We consider a generic probabilisitc model in the form of $\p(\mathcal{T},\mathcal{Z})=\p(\mathcal{T}|\mathcal{Z})\p(\mathcal{Z})$. Our objective is to find an approximation to the intractable posterior distribution $p(\mathcal{Z}|\mathcal{T})$. Let $\q{\phi}$ denote the variational posterior distribution parameterized with $\phi$. We further set
\begin{align}
f_{\phi}(\mathcal{Z})=\log \p(\mathcal{T},\mathcal{Z}) - \log \q_{\phi}(\mathcal{Z}).
\end{align}
The ELBO is thus given by
\begin{align}
\mathrm{ELBO} = \e[\log \p(\mathcal{T},\mathcal{Z})-\log \q_{\phi}(\mathcal{Z})]=\e[f_{\phi}(\mathcal{Z})].
\end{align}
Recall that we are now interested in situations where it is no longer possible to compute the required expections under $\q$ analytically. The objective is to maximize the ELBO. The mechanics is simple: We first differentiate the ELBO w.r.t. the variational parameter. The resulting gradient is represented as an expectation which is then evaluated using Monte Carlo techniques, i.e. by sampling from the variational distribution and forming the corresponding Monte Carlo estimates of the gradient. Differentiating the ELBO w.r.t. $\phi$, we get
\begin{align}
\label{eq:temp1}
\frac{\partial}{\partial \phi}\mathrm{ELBO} = \frac{\partial}{\partial \phi}\e[f_{\phi}(\mathcal{Z})].
\end{align}
We shall represent the above gradient of expectation as the expectation of the gradient.  Computing
the gradient w.r.t. $\phi$ needs extra attention since the expectation is being taken w.r.t. $\q$ and thus we cannot simply swap the gradient with the expectation. Two standard techniques in evaluating the gradient results in two different estimators in the literature:
\begin{itemize}
	\item \textbf{Score function estimator.} Here the gradient of the ELBO is expressed as an expectation with
	respect  to  the  variational  distribution  using  the  log-derivative  trick, nder which the Lebesgue’s dominated convergence theorem becomes applicable so that we can take the gradient of the expectation above by moving the gradient inside the expectation.  It then takes samples from the variational distribution to calculate noisy gradients. This is the method introduced in \cite{ranganath2014black}.
	\item \textbf{Pathwise gradient estimator.} This method is based on the reparameterization trick. This approach reparameterizes the latent variable $z$ in terms of a set of auxiliary variables $\epsilon$ with a recognizable distribution $\p(\epsilon)$ which does not depend on the variational parameters. This means that the expectation in (\ref{eq:temp1}) can now be taken w.r.t. $\p(\epsilon)$ as opposed to $\q$ which then enables us to simply move the gradient inside the expectation. This procedure only requires drawing samples from $\p(\epsilon)$. This method was first introduced by \cite{figurnov2018implicit}.
\end{itemize}

In this work, we use the method of pathwise gradient estimator.

\begin{algorithm}[!ht]
	\caption{Black-Box Variational Inference}
	\label{algo:bbvi}
	\textbf{Input:} $\theta$ is the set of parameters of the model, $T$ is the time maturity.\\
	\textbf{Output:} simulated event times
	\begin{algorithmic}[1]
		\State Initialize $\phi$
		\Repeat 
		\For{$l=1$ to $L$}
		\State Sample $\mathcal{Z}^{(l)} \sim \q_\phi(\mathcal{Z})$.
		\EndFor
		
		\State Update variational parameters:
		\begin{align}
		&\mathrm{ELBO}(\phi) \approx L^{-1}\sum_{l=1}^L\Big(\p(\mathcal{T}, \mathcal{Z}^{(l)}) - \q_\phi(\mathcal{Z}^{(l)})\Big)\\
		&\phi \leftarrow \phi + \eta \times \frac{\partial}{\partial \phi}\mathrm{ELBO}(\phi)
		\end{align}
		\Until {converged}
	\end{algorithmic}
	
\end{algorithm}

\section{Thinning Algorithm for Simulation of Point Processes}
Algorithm~\ref{algo:point-process} presents thinning algorithm by \cite{ogata1981lewis} for simulation of general point processes. We use this algorithm to simulate Hawkes, NL-Hawkes, and HPP. To simulate S-Hawkes process, we modify algorithm to add stochastic level of excitation (Algorithm~\ref{algo:point-process-stochastic}).

\begin{algorithm}[!ht]
	\caption{Simulation of Point Process (Hawkes, NL-Hawkes, HPP)}
	\label{algo:point-process}
	\textbf{Input:} $\theta$ is the set of parameters of the model, $T$ is the time maturity.\\
	\textbf{Output:} simulated event times
	\begin{algorithmic}[1]
		\State Initialize $\mathcal{T} = \emptyset, s=0, n=0$
		\While {$s<T$}
		\State Set $\bar{\lambda} = \lambda(s; \theta)$
		\State Sample $u \sim \text{Uniform}(0,1)$
		\State Let $w = -\log u/\bar{\lambda}$
		\State Set $s = s + w$
		\State Sample $v \sim \text{Uniform}(0,1)$
		\State Let $\lambda_s = \lambda(s; \theta)$
		\If {$v\bar{\lambda} \le \lambda_s$}
		\State $n = n+1$
		\State $t_n = s$
		\State $\mathcal{T} = \mathcal{T} \cup \{t_n\}$
		\EndIf
		\EndWhile
		\If {$t_n \ge T$}
		\State $\mathcal{T} = \mathcal{T}\backslash\{t_n\}$
		\EndIf
		
		\State \Return $\mathcal{T}$
	\end{algorithmic}
	
\end{algorithm}

\begin{algorithm}[!ht]
	\caption{Simulation of S-Hawkes Process}
	\label{algo:point-process-stochastic}
	\textbf{Input:} $\theta = \{\mu, \beta, \delta\}$ is the set of parameters of the model, $T$ is the time maturity.\\
	\textbf{Output:} simulated event times
	\begin{algorithmic}[1]
		\State Initialize $\mathcal{T} = \emptyset, \mathcal{J} = \emptyset, s=0, n=0$
		\While {$s<T$}
		\State Set $\bar{\lambda} = g(t) + \sum_{j: t_j\in\mathcal{T},\alpha_j\in \mathcal{J}}\alpha_j e^{-\delta(s-t_j)}$
		\State Sample $u \sim \text{Uniform}(0,1)$
		\State Let $w = -\log u/\bar{\lambda}$
		\State Set $s = s + w$
		\State Sample $v \sim \text{Uniform}(0,1)$
		\State Let $\lambda_s = g(t) + \sum_{j: t_j\in\mathcal{T},\alpha_j\in \mathcal{J}}\alpha_j e^{-\delta(s-t_j)}$
		\If {$v\bar{\lambda} \le \lambda_s$}
		\State $n = n+1$
		\State $t_n = s$
		\State $\mathcal{T} = \mathcal{T} \cup \{t_n\}$
		\State Sample $a_n \sim \text{Exponential}(\alpha\mid\beta)$
		\State $\mathcal{J} = \mathcal{J} \cup a_n$
		\EndIf
		\EndWhile
		\If {$t_n \ge T$}
		\State $\mathcal{T} = \mathcal{T}\backslash\{t_n\}$
		\State $\mathcal{J} = \mathcal{J}\backslash\{a_n\}$
		\EndIf
		
		\State \Return $\mathcal{T}$
	\end{algorithmic}
	
\end{algorithm}
\section{Variational Evidence for Stochastic Hawkes Process}
Stochastic Hawkes process \cite{lee2016hawkes} is a generatization of Hawkes process with the size of excitation is a stochastic process. An example of stochastic Hawkes process is as follows:
\begin{align}
&\lambda(t) = \mu + (\lambda_0 - \mu)e^{-\delta t} + \sum_{j:T_j<t}\alpha_j e^{-\delta(t-T_j)}\\
&\alpha_j \sim \text{Exponential}(\alpha\mid b_\alpha)
\end{align}
Unlike classical Hawkes process where $\alpha$ is a constant, stochastic Hawkes models $\alpha$ as a random variable; so at each event time, the level of excitations is different from the previous event time. Under Bayesian setting, the set of latent variables is $\mathcal{Z} = \{\mu, \delta, \alpha_1,\dots,\alpha_{N(T)}, b_\alpha\}$. We set the priors and variational posterior distribution for $\mu>0, \delta>0, \alpha_j>0, b_\alpha>0$ in Stochastic Hawkes as log-normal distributions: $\q^\star(\mu) = \text{Log-}\mathcal{N}(\mu\mid m_\mu, \exp(s_\mu)^2)$, $\q^\star(\alpha) = \text{Log-}\mathcal{N}(\alpha\mid m_\alpha, \exp(s_\alpha)^2)$, $\q^\star(\delta) = \text{Log-}\mathcal{N}(\delta\mid m_\delta, \exp(s_\delta)^2)$, $\q^\star(b_\alpha) = \text{Log-}\mathcal{N}(b_\alpha\mid m_b, \exp(s_b)^2)$, where $\{m_\mu, m_\alpha,m_\delta,m_b,s_\mu,s_\alpha,s_\delta, s_b\}$ are the parameters to be estimated. Under this setting, we learn the parameters by maximizing 
\begin{align}
&\mathcal{L}_{SH} = L^{-1}(G_1 + G_2 - G_3)\\
&G_1 = \sum_{i=1}^{N(T)}\log\lambda^{(l)}(T_i) - \int_0^T\lambda^{(l)}(s)\,ds\\
&G_2 = -\log\mu^{(l)} - \frac{(\log\mu^{(l)})^2}{2} - N(T)\log b_\alpha^{(l)} - \sum_{j=1}^{N(T)}\frac{\alpha_j^{(l)}}{b_\alpha} -\log\delta^{(l)} - \frac{(\log\delta^{(l)})^2}{2}-\log b_\alpha^{(l)} - \frac{(\log b_\alpha^{(l)})^2}{2}\\
&G_3 = -s_\mu -\log\mu^{(l)}- \frac{(\log\mu^{(l)} - m_\mu)^2}{2\exp(s_\mu)^2} -s_\delta -\log\delta^{(l)}- \frac{(\log\delta^{(l)} - m_\delta)^2}{2\exp(s_\delta)^2}-N(T)s_\alpha- \sum_{j=1}^{N(T)}\frac{(\log\alpha_j^{(l)} - m_\alpha)^2}{2\exp(s_\alpha)^2}\nonumber\\
&\qquad -s_b -\log b_\alpha^{(l)}- \frac{(\log b_\alpha^{(l)} - m_b)^2}{2\exp(s_b)^2}
\end{align}
with $\mu^{(l)}, \alpha_j^{(l)}, a_\alpha^{(l)}, b_\alpha^{(l)}, \delta^{(l)}$ are sampled from variational distribution using reparameterization: $\mu^{(l)} = \exp(m_\mu + \exp(s_\mu)\epsilon_\mu^{(l)})$, $\alpha^{(l)} = \exp(m_\mu + \exp(s_\alpha)\epsilon_\alpha^{(l)})$, $\delta^{(l)} = \exp(m_\delta + \exp(s_\delta)\epsilon_\delta^{(l)})$ where $\epsilon_\mu^{(l)} \sim \mathcal{N}(0,1)$, $\epsilon_\alpha^{(l)} \sim \mathcal{N}(0,1)$, and $\epsilon_\delta^{(l)} \sim \mathcal{N}(0,1)$, $\lambda^{(l)}(\cdot)$ is the intensity computed with samples $\mu^{(l)}, \alpha^{(l)}, \delta^{(l)}$. Notice that when we set $\alpha_j$ as a constant, we retrieve back classical Hawkes process.
\section{Variational Evidence for Nonlinear Hawkes Process}
A nonlinear Hawkes process is a counting process driven by the following intensity:
\begin{align}
&\lambda(t) = \mathcal{S}\bigg(\mu + \left(\lambda_0 - \mu\right)e^{-\delta t} + \sum_{T_j \in \mathcal{H}_t}\alpha e^{-\delta\left(t- T_j\right)}\bigg)
\end{align}
where $\mathcal{T} = \{T_1, \dots, T_{N}\}$ is set of event times, $\mathcal{H}_t$ is the set of event history up to time $t$, i.e. $\mathcal{H}_t = \{T_j \in \mathcal{T}|T_j < t\}$, $\{\mu, \alpha,\delta\}$ is the set of parameters, $\mathcal{S}(\cdot):\mathbb{R} \rightarrow \mathbb{R}^+$ is a link function such as linear: $\mathcal{S}(x) = x$, soft plus: $\mathcal{S}(x) = \log(1 + \exp(x))$, exponential: $\mathcal{S}(x) = \exp(x)$. Note that when $\mathcal{S}(\cdot)$ is linear, we retrieve back the classical Hawkes process. One characteristic of nonlinear Hawkes process is that it allow exhibition excitation, i.e. the moment an event happens, the rate $\lambda(t)$ maybe increase, so $\mu \in \mathbb{R}, \alpha \in \mathbb{R}, \delta > 0$. Based on these restriction, we propose the variational distributions for $\mu, \alpha, \delta$ as follows:
\begin{align}
\q^\star(\mu) &= \mathcal{N}(\mu\mid m_\mu, \exp(s_\mu)^2)\\
\q^\star(\alpha) &= \mathcal{N}(\alpha\mid m_\alpha, \exp(s_\alpha)^2)\\
\q^\star(\delta) &= \text{Log-}\mathcal{N}(\delta\mid m_\delta, \exp(s_\delta)^2)
\end{align}
where $\{m_\mu,m_\alpha,m_\delta,s_\mu,s_\alpha,s_\delta\}$ is the set of parameters to be learned by maximizing the ELBO
\begin{align}
&\mathcal{L}_{NH} = L^{-1}(G_1 + G_2 - G_3)\\
&G_1 = \sum_{i=1}^{N(T)}\log\lambda^{(l)}(T_i) - \int_0^T\lambda^{(l)}(s)\,ds\\
&G_2 =  - \frac{(\mu^{(l)})^2}{2}  - \frac{(\alpha^{(l)})^2}{2} -\log\delta^{(l)} - \frac{(\log\delta^{(l)})^2}{2}\\
&G_3 = -s_\mu- \frac{(\mu^{(l)} - m_\mu)^2}{2\exp(s_\mu)^2} -s_\alpha- \frac{(\alpha^{(l)} - m_\alpha)^2}{2\exp(s_\alpha)^2} -s_\delta - \log\delta^{(l)}- \frac{(\log\delta^{(l)} - m_\delta)^2}{2\exp(s_\delta)^2}
\end{align}
with $\mu^{(l)}, \alpha^{(l)}, \delta^{(l)}$ are sampled from variational distribution using reparameterization: $\mu^{(l)} = m_\mu + \exp(s_\mu)\epsilon_\mu^{(l)}$, $\alpha^{(l)} = m_\mu + \exp(s_\alpha)\epsilon_\alpha^{(l)}$, $\delta^{(l)} = \exp(m_\delta + \exp(s_\delta)\epsilon_\delta^{(l)})$ where $\epsilon_\mu^{(l)} \sim \mathcal{N}(0,1)$, $\epsilon_\alpha^{(l)} \sim \mathcal{N}(0,1)$, and $\epsilon_\delta^{(l)} \sim \mathcal{N}(0,1)$, $\lambda^{(l)}(\cdot)$ is the intensity computed with samples $\mu^{(l)}, \alpha^{(l)}, \delta^{(l)}$.
\section{Additional Experimental Results on Synthetic Data}
Figure~\ref{fig:convergence-parameters} presents convergence of each parameters in synthetic data. Figure~\ref{fig:bf-synthetic-full} shows VBF on different true models. In general, the more observed data, the higher evidence that it comes from the true model.
\begin{figure}[!ht]
	\begin{center}
		\includegraphics[width=0.75\textwidth]{figures/variational-distributions-full}
		\caption{Variational posterior distribution (using BBVI) and the true posterior (sampling with MCMC) of parameters on Hawkes, Stochastic Hawkes, Nonlinear Hawkes, and HPP. In general, our model is good when posterior coincides with the variational distribution. As we see, the graphs of true posterior and variational distributions roughy coincides, this reasures that our BBVI is good enough to approximate the posterior.}\label{fig:calibrate-hawkes-full}
	\end{center}
	\vskip -0.2in
\end{figure}
\begin{figure}
	\begin{center}
		\includegraphics[width=0.9\textwidth]{figures/convergence-parameters}
		\caption{Convergence of parameters on Hawkes, Stochastic Hawkes, Nonlinear Hawkes, and HPP. The figures show that each parameter starts to converge after a certain iteration.}\label{fig:convergence-parameters}
	\end{center}
	\vskip -0.2in
\end{figure}
\begin{figure}
	\begin{center}
		\includegraphics[width=0.97\textwidth]{figures/true-model-full}
		\caption{Variational evidence and VBF on different true model: Hawkes, Stochastic Hawkes, Nonlinear Hawkes, HPP. The first column shows that variational evidence of the true model is higher than the other models. The second, third, and fourth columns show VBF of true model over the other models; in general, the more observed event times, the higher evidence that it comes from the true model.}\label{fig:bf-synthetic-full}
	\end{center}
	\vskip -0.2in
\end{figure}
\section{Additional Experimental Results on Earthquakes Data}
In this section, we present some additional results on convergence of parameters on earthquakes data. Figure~\ref{fig:convergence-parameters-earthquakes0},~\ref{fig:convergence-parameters-earthquakes1} present the value of each parameter in each iteration.
\begin{figure}
	\begin{center}
		\includegraphics[width=0.9\textwidth]{figures/earthquakes-convergence-parameters0}
		\caption{Convergence of parameters on earthquakes data in Kwanto. The figures show that each parameter starts to converge after a certain iteration.}\label{fig:convergence-parameters-earthquakes0}
	\end{center}
	\vskip -0.2in
\end{figure}

\begin{figure}
	\begin{center}
		\includegraphics[width=0.9\textwidth]{figures/earthquakes-convergence-parameters1}
		\caption{Convergence of parameters on earthquakes data in Hida. The figures show that each parameter starts to converge after a certain iteration.}\label{fig:convergence-parameters-earthquakes1}
	\end{center}
	\vskip -0.2in
\end{figure}
